# Supplementary material for: On Bridging the Gap between Mean Field and Finite Width in Deep Random Neural Networks with Batch Normalization
Source: arXiv:2205.13076 source file (2023-02-20)
Supplement: Supplementary file 1 [file Gaussian_product.tex]

\section{Gaussian product analysis}\label{app:Gaussian_prod_conditioning}
\textit{Details (can move to appendix)}
We used the fact that for positive-definite square matrices $A B$ has same spectrum as $B A$ to rewrite this as $\E \det(X^\top X) \det(\prod_k^\ell G_k^\top G_k).$ Using the fact that $\det(A B) = \det(A)\det(B)$, we arrive at $\E \prod_k^\ell \det(G_k^\top G_K)$. Which because of Independence of $G_k$'s decomposes to yield $\det(C_\ell) = \det(X^\top X) \prod_k^\ell \E \det(G_k^\top G_k)=\prod_k^\ell \E \det(G_k^\top G_k),$ where we used $\det(X^\top X)=\det(I_n)=1.$ Invoking results known for Wishart matrices\cite{}, $\E \det(G_k^\top G_k)\lesssim 1-n^2d^{-1}.$ Using the numerical inequality $1+x\le \exp(x)$, we can summarise the result to $\E \det(C_\ell)\le \det(X^\top X)\exp(-c n^2 \ell d^{-1})$ for some absolute constant $c$

In summary, we have shown that the discrepancy of shallow and deep mean field rises from a mere possibility to an eventuality in the case of vanilla MLP with identity activation. We shall note that these aer not necessarily universal results for all activation functions. Notably, ~\cite{li2021future,li2022neural} show that shaping activation is one way of stabilizing the representations to the effect of accurately predicting the distribution of gram matrix in infinite depth regime. However, the focus of the current work is the study of effects of normalization for activations that exhibit varying degrees of discrepancy under shallow and deep mean field. To the best of our knowledge, this topic has not received a theoretical and principled treatment, and we will attempt to give such a treatment in the following section.
