# Supplementary material for: On Bridging the Gap between Mean Field and Finite Width in Deep Random Neural Networks with Batch Normalization
Source: arXiv:2205.13076 source file (2023-02-20)
Supplement: Supplementary file 2 [file divergence.tex]

\section{Distortion}\label{app:distortion}

The first term $\norm{\C^{-1}}$ captures the conditioning of matrix $\C$ and the rate of convergence \textcolor{blue}{Convergence of a a constant matrix? } of the scatter matrix to the second moment. Namely, if $x_1,\dots, x_d\sim\mu$ with second moment $\mathbb{E}\mu xx^\top=\C$, the convergence of $\frac{1}{d} \sum_i x_i x_i^\top$ to $\C$ as a function of $d$, depends on the smallest eigenvalue of $\C$. Since the Batch Normalization (BN) operator always projects points onto a sphere with $\sqrt{n}$ radius, the distortion of the sphere captures the largest possible value of $\F(\BN(x))$. Therefore, the distortion of the sphere by the activation function $\F$ captures the convergence rate induced by the activation function \textcolor{blue}{Activation induces convergence?}, when applied after normalization.
Now we present the main theorem that characterizes the stability of Batch Normalization (BN)-MLP networks, and a corollary that describes the divergence between two independent copies of the same BN-MLP network.

Note that scaling $F$  by a constant will inversely scale $\C^\nhalf$ by a similar constant. Therefore, the distortion is a scale-invariant constant and distortion of $F(x)$ automatically transfers to all activations $\{a F(x): a\in\R\}$.  
If we assuming that the stable second moment $\C$ is well-conditioned $\norm{\C^{-1}}=\mathcal{O}(1)$,we only need to show that $F$ does not arbitrarily ``stretch'' the $\sqrt{n}$-sphere to prove constant distortion $\distort$. For example, if $F(x)$ is linearly bounded by $F(x)\le |x|$, the stretch of sphere is also bonded by $1$. 

\section{Divergence}\label{sec:divergence}

Note that if $\lambda_i$'s are eigenvalues of $C_1 C_2^{-1}$, then the divergence is equal to $\sum_i^n(\lambda_i-1)^2$. Therefore, $\couple(C_1,C_2)=0$ implies that $C_1 = C_2^{-1}$. The main motivation behind definition of $\couple$ is that it provides a lower and upper bound on a total variation of multivariate Gaussian: $\frac{1}{100}\couple(C_1,C_2)\le \norm{\mu_X-\mu_Y}_{tv}\le \frac32\couple(C_1,C_2)$, when $X\sim\Normal(0,C_1)$ and $Y\sim\Normal(0,C_2)$.
