# Supplementary material for: On Bridging the Gap between Mean Field and Finite Width in Deep Random Neural Networks with Batch Normalization
Source: arXiv:2205.13076 source file (2023-02-20)
Supplement: Supplementary file 3 [file ergodicity.tex]

\section{Geometrically Ergodic Assumption }\label{app:ergodicity}
Recall that for an ergodic Markov chain $\T$, given enough number of steps, it converges to a invariant distribution $\lim_{k\to\infty} \T^k_\#(\mu_0) = \mu_\infty,$ where $\mu_0$ and $\mu_\infty$ are respectively initial and invariant. We can restate this in terms of total variation $\lim_{k\to\infty}\TV(\mu_\infty,\T^k_\#(\mu_0))=0$. Crucially, invariant does not depend on the initial distribution $\mu_0.$  
% This implies that given two copies of the same chain $\{H_k\}$ and $\{H'_k\}$, we must also have $\TV(H_k,H'_k)=0$ as $k\to\infty.$ This latest formulation is of particular interest, because it allows us to analyze stability by looking at behavior of two independent copies of the same chain. 
The distinctive feature of invariant is that, it enables us to make non-vacuous statements about invariant will transfer to infinite depth, even when width is finite. This stands in contrast to to union type bounds that become vacuous in depth. The difficulty, however, is in establishing ergodicity over the chain or some mapping of the probability space. 

For reasons outlined previously, we are interested in spectral properties in gram matrix. Let us highlight the importance of ergodicity by an example where gram matrices of a vanilla MLP with identity activations $X_k = G_k X_{k-1}$ with $X_0\in R^{d\times n}$ as input and Gaussian products with iid elements from $\Normal(0,1/d)$. 
% \textit{Gaussian product chain is not ergodic.} 
In the previous section we established that the product of Gaussian matrices has expected poor conditioning $\exp(n\ell/2d).$ In fact, stronger statements can be made in~\cite{bougerol2012products}, that imply the product converges to a rank-1 matrix: $\prod_k^\ell G_k \to u\otimes v$ up to some scale, where $u_k,v_k\in\R^n$ are singular vectors with orientation in $\R^d, $. Observe that the product of $X_k^\top X_k$ is distributed as $(u_k v_k^\top X_0 )^\top (u_k v_k^\top X_0) = (v_k^\top X_0)^\top (v_k^\top X_0)$ up to some scale. Because $v_k$ is has random orientation that is dictated at each step independently $G_k$, the distribution of $X_k^\top X_k$ cannot have a distribution in the limit $k\to\infty$. In particular, the distribution of the norm $\norm{v_k^\top X_0}$ depends on the spectral distribution of $X_0$, which violates the requirement that the stationary does not depend on the input.
In fact, much broader non-ergodicity results can are implied by theories developed by Furstenberg~\cite{furstenberg1963noncommuting}, showing that very special cases of matrix products are ergodic, which does not include Gaussian products. \textcolor{blue}{double check this.} 
If we assume the contra-positive that $\mu_\infty(X_k^\top X_k)$ exists, we can conclude that $\lim_{k\to\infty} \TV(\mu_\infty,\mu_{y_k})\neq 0$ which violates the definition of invariant.

One can observe that norm of these vectors $x_k^\top x_k=\norm{x_k}^2$ has a remarkably simple form. In fact, because the distribution Gaussian matrix products are isotropic, the distribution of $\norm{x_k}^2$ is fixed up to a scaling with $\norm{x_0}^2.$

\textit{Random walk on the sphere.} Now let us analyze the Gaussian product chain where at every step we project the input from previous step onto the unit sphere: $\hat{x_k}=x_k/\norm{x_k}$ with $x_k = G_k \hat{x}_{k-1}.$ Observe that the chain $\{x_k\}$ can be alternatively viewed as a random walk on the unit sphere $x_k = U_k x_{k-1}$, where $U_k$ is a uniformly drawn orthonormal matrix $U_k^\top U_k = I_d.$ Let $\{x_k\}$ and $\{y_k\}$ be two copies of the same chain, with respective random rotation matrices $\{U_k\}$ and $\{V_k\}.$

Despite these elegant properties of of a random walk on the sphere, this example does not correspond to MLP chain with batch normalization, which is the topic of next section.

\paragraph{Ergodicity of gram matrices in MLP with batch normalization.}
In our main case study that is the BN-MLP chain, extensive experiments and numerical validation that this chain of the gram matrices is ergodic under a wide range of activation and finite width and batch sizes. However, to the best of our knowledge, there is currently no analysis and rigorous of this chain. We conjecture this that such a contraction in total variation of gram matrices exists, and will provide experimental and theoretical insight for why this is the case.

Building on the mean field theory approach, we utilize tools from the theory of Markov chains to study the invariant of hidden representation matrices across the layers of the network.

\paragraph{Analysis of Gaussian product chain with normalization}

Let us modify the previous example by adding normalization, with identity activations $\widehat{X_k} = \BN(X_k)$ where $X_k = G_k \widehat{X}_{k-1}$, and $\BN(X)$ is defined as projecting rows on to the unit sphere $\BN(X)_{i\cdot} = X_{i\cdot}/\norm{X_{i\cdot}}$. Let us consider the gram matrix sequence $C_k:=\widehat{X}_k^\top \widehat{X}_k$. Observe that the trace of the gram matrix has a remarkably simple form $\tr(\E C_k)=\E \tr( \widehat{X}_k^\top \widehat{X}_k) = \E \frac1d \sum_i^d \norm{(\widehat{X}_k)_{i\cdot}}^2  = 1.$ Therefore, we can measure the behavior by tracking the determinant $\det(C_k).$ By log-concavity property of log-determinant, we have $\log\det(\E C_k) \ge \E \log\det(C_k)$. 
Let us consider a single step of the chain as $C = \BN(G X)^\top \BN(G X).$ 
Observe that we can write the gram matrix as $C = D^{-1} S D^{-1}$, where $S$ is the gram matrix of non-normalized matrix $S=(G X)^\top (G X)$, and $D$ is a diagonal matrix with inverse norms of each row $D = \diag(\norm{(GX)_{i\dots}}_{i\le d}).$ By product decomposition property of determinant, $\det(C)=\det(D)^{-2}\det(S)$. Because $D$ is diagonal, we have $\log\det(D) = \sum_{i\le d}\log\norm{(GX)_{i\cdot}}$.  Furthermore, we have $ S = X^\top G^\top G X$. By properties determinant, we have $\log\det(S)=\log\det(G^\top G)+\log\det(X^\top X).$  Overall, we have $\log\det(C) = -2\sum_{i\le d}\log\norm{(GX)_{i\cdot}} + \log(G^\top G) + \log\det(X^\top X)$. Furthermore, rows of $GX $ are all identically distributed from $\Normal(0,
\frac1d X^\top X)$. Therefore, $\norm{(GX)_{i\cdot}}^2$ is distributed as a weighted sum of chi-squared random variables, with eigenvalues of $\frac1d X^\top X$ as weights.
