# Supplementary material for: On Bridging the Gap between Mean Field and Finite Width in Deep Random Neural Networks with Batch Normalization
Source: arXiv:2205.13076 source file (2023-02-20)
Supplement: Supplementary file 4 [file stable.tex]

\section{Mean Field Theory for Deep Neural Networks with Batch Normalization}

% \cite{yang2019mean} We are particularly interested in understanding the hidden representations of input samples at each layer, which they denote as $H_\ell\in \R^{d\times n}$. We consider two types of normalization layers, projection normalization and standard batch normalization, and prove a conjecture on stable Gram matrices for a broad range of activation functions. We build upon the mean-field framework introduced by a previous study to understand the behavior of deep neural networks with batch normalization. We show that as the width of the network tends towards infinity, the Gram matrix of the hidden representation follows a recurrence relation, and the fixed point of this relation provides valuable insights into the spectra of the hidden representations. The stable Gram matrix is unique and has a particular structure due to the symmetry of the neural architecture.
% In this section, we review mean-field analysis for random deep neural networks with batch normalization. 
\paragraph{The chain of representations.}
Consider the hidden representations of input samples at each layer denoted by $H_\ell\in \R^{d\times n}$. The input batch is represented by $H_0$. These hidden representations construct a Markov chain of random matrices as
\textcolor{blue}{Let's finalize these notations. Please avoid defining the same notation in the next chapter. }
\begin{align}
H_{\ell+1}:=\frac{1}{\sqrt{d}}W_\ell T(H_\ell), \quad T(M) :=  \F \circ \normop (M),
\end{align}

where $\F$ is the element-wise activation function, ${W_\ell \in \R^{d\times d}}$ are random weight matrices with i.i.d. Gaussian elements, and $\normop$ denotes the batch normalization layer that operates row-wise: $[\normop(A)]_{i.} = \normop(A_{i.}).$ We consider two types of normalization layers: projection normalization ($\bn$) and standard batch normalization ($\BN$):
\begin{itemize}
    \item Projection $\bn$ maps $\R^n$ onto the $n$-sphere with radius $\sqrt{n}$ by dividing the input vector by its norm: $\bn(v) := \frac{v}{\sqrt{\frac1n\sum_i v_i^2}}$. This type of normalization has been used in previous studies~\cite{daneshmand2020batch,daneshmand2021batch}. 
    \item Normalization $\BN$ centering and normalizing $\R^n$ centers the input vector and then performs length normalization: $\BN(v) := \bn\left(v-\frac1n \sum_i^n v_i\right)$. This normalization is the standard batch normalization proposed by \cite{ioffe2015batch}.
\end{itemize}

In this section, we review the mean field framework introduced by\cite{yang2019mean} to understand the behavior the Gram matrices $C_\ell = H_\ell^\top H_\ell$ with $\ell$. \textcolor{blue}{we need to talk about the mean-field result once. I recommend to present mean-field results first and show experimentally they are predictive. We can first present the exact result form \cite{yang2019mean} Then, experimentally substantiate it for network with finite widths. Then we say that we want to bridge this Gap. I could not understand your pointers about the convergence of the covariance to move it here.}

As the width of the network tends towards infinity, the Gram matrix of the hidden representation, denoted by $C_\ell = H_\ell^\top H_\ell$, follows the recurrence relation:
\begin{align} \label{eq:mdynamics}
C_{\ell+1} = h(C_\ell)
\end{align}

where $h:\R^{n\times n} \to \R^{n\times n}$ is obtained by taking the expectation over Gaussian random variables:
\begin{align*}
h(C) := \E_\rvw\left[\phi(\rvw ) \phi(\rvw )^{\top} \right] = \Cst, \quad \rvw\sim\Normal(\0_n,\Cst)
\end{align*}

for $\phi:=\F\circ\normop$. This expectation resembles the limit of the network width tending towards infinity. By taking the expectation, the dynamics of $H_\ell^\top H_\ell $ become deterministic. However, the dynamics of $C_\ell$ are difficult to analyze \cite{yang2019mean}.

The fixed point of equation \ref{eq:mdynamics} provides valuable insights into the spectra of the hidden representations. A fixed point $\Cst \in \R^{n\times n}$ satisfies $h(\Cst) = \Cst$. We refer to this fixed point as the stable Gram matrix associated with the neural network. \cite{yang2019mean} prove that the stable Gram matrix is unique and has a particular structure due to the symmetry of the neural architecture. Specifically, there exist constants $\alpha$ and $q$ such that:
\begin{align}
\Cst = \beta ( (1-\rho) I_n + \rho \1_{n\times n})
\end{align}

The choice of the parameter $\rho$ has a strong influence on the spectrum of $\Cst$. When $\rho=0$, $\Cst$ is a full rank matrix, while $\rho=1$ results in a low rank matrix structure. Thus, it is important to determine the value of $\rho$. For networks with linear activations, \cite{yang2019mean} prove that $\rho=0$. Based on numerical simulations, ~\cite{yang2019mean} conjecture that this result holds for a wide range of activation functions. ~\cite{yang2019mean} propose the following conjecture:

\begin{conjecture}{\cite{yang2019mean}} \label{con:mean_field}
The stable Gram matrix $\Cst$ is a scaling factor of the identity matrix for networks with ReLU, hyperbolic tangent, leaky ReLU, and sigmoid activations.
\end{conjecture}

In the following subsection, we prove this conjecture holds true for networks with a broad range of symmetric activation functions, including hyperbolic tangent and sine activations.

In this section, we provide evidence that the stable Gram matrix for deep neural networks with batch normalization and a broad range of activation functions can be well-approximated by the mean field framework.

First, we prove Conjecture \ref{con:mean_field} for symmetric activation functions:
\begin{lemma}[Proof of Conjecture~\ref{con:mean_field} for symmetric activations]\label{lem:odd_C}
Suppose $ \F(-a) = -\F(a)$ holds for all $a$ and define $\phi:=\F\circ \bn$. Then, $\Cst:=\beta_F I_n$ with
\begin{align} \label{eq:bf}
\beta_F &:= \Expec{\F^2\left(\nfrac{\rvw_1}{\sqrt{\frac{1}{n}\sum_{j=1}^n \rvw_{j}^2}}\right)},
\end{align}
where $\rvw_i$ are i.i.d. standard Gaussian random variables.
\end{lemma}

This result shows that the rank of $C_\ell$ does not collapse as $\ell \to \infty$, which is not just a theoretical result. Daneshmand et al. (2020, 2021) argue that avoiding rank collapse is strongly linked to improved training with batch normalization layers. Thus, this mean field analysis provides insights into the training of neural networks with finite width.

Note that the ReLU activation does not satisfy the symmetric property required in Lemma \ref{lem:odd_C}. For the ReLU activation, we establish a bound on the constant \begin{lemma}\label{lem:relu_C}
\label{prop:relu} For activation $\relu(x):=\max(0,x)$ and normalization $\BN$, there exists $0\le \rho \le \frac12$, such that 
\begin{align*}
\Cst:=\frac12(1-\rho) I_n + \frac\rho2 \1_{n\times n}.
\end{align*}
\end{lemma}

This result shows that the eigenvalues of $\Cst$ lie in the range $[\frac{1}{4},1]$, making it a well-conditioned matrix. The proof is based on an application of Brouwer's fixed point theorem. We believe this proof technique can be used to estimate the spectrum of the stable Gram matrix for a wide range of non-linear activation functions.

\subsection{Finite Width vs. Infinite Width}

The precise characterization of the stable Gram matrix in the previous lemmas allows us to experimentally validate whether these results extend to networks with finite width. To do this, we choose a wide network and show that the eigenvalues of $H_\ell^\top H_\ell$ lie in the range $[\nfrac14,1]$ for the ReLU activation. For the hyperbolic tangent activation, our plot in Figure 2 (after slight modifications) is sufficient to demonstrate this result.

[TODO: Insert specific details and results for the experimental validation.]
