# Supplementary material for: On Bridging the Gap between Mean Field and Finite Width in Deep Random Neural Networks with Batch Normalization
Source: arXiv:2205.13076 source file (2023-02-20)
Supplement: Supplementary file 5 [file recap.tex]

\section{Recap of related concepts}
\paragraph{Linear Algebra Recap: SVD and Eigenvalue Decomposition \textcolor{blue}{reduced/removed?}}
Given a matrix $M\in \R^{n\times m}$, its reduced singular value decomposition (SVD) refers to orthogonal matrices $U\in\R^{m\times r}$, $V\in\R^{n\times r}$ such that $U^\top U = V^\top V = I_r$ and a diagonal matrix $S\in\R^{r\times r}$, such that $M = U S V^\top$, with $U$ and $V$ as eigenvectors, and $\diag(S)=(s_1,\dots,s_n)$ denoting the singular values $s_1\ge \dots \ge s_n\ge 0$. For symmetric matrices $M$, this simplifies to eigenvalue decomposition $M = U \Lambda U^\top$, where $U$ are eigenvectors, respectively, and $\diag(\Lambda)$ contains the singular values $\lambda_1\ge \dots\ge \lambda_n$. If all eigenvalues of $M$ are positive (non-negative), it is positive definite (semi-definite), denoted by $M\succ 0$ ($M \succeq 0$). For positive definite $M$, its powers are defined as $M^\alpha = U S^\alpha U^\top$. We use the notation $\norm{C}$ to denote the $L^2$ operator norm of any operator $T\colon\R^n\to\R^n$: $\norm{T}=\sup_{x\in\R^n}\norm{T(x)}/\norm{x}$. In the special case of $T(x)=M x$ for a positive definite $M\in\R^{n\times n}$, this is equal to its largest singular value $s_1(M)$. We use $\kappa(C)$ to denote condition number $\kappa(C)=\norm{C}\norm{C^{-1}},$ defined for non-singular matrices. 

% In our analysis, we frequently use the fact that for symmetric matrices $A, B\in\R^{n\times n}$, the singular decomposition of $A B$ is similar to $B A$.
